# Supplementary material for: Deterministic and Reliable Software-Defined Vehicles: key building blocks, challenges, and vision
Source: arXiv:2407.17287 source file (2025-01-09)
Supplement: Supplementary file 1 [file appendix.tex]

%%%%%%%%%%%%%%%%%%%%%%%%%%
\chapter{Research methodology}
\label{appendix:sota-methodology}

The research methodology started with a search based on the topics defined in~\cref{sec:sota-methodology} and~\cref{sec:background-methodology}, which were researched within 3 queries:
\footnotesize{
	\begin{itemize}
    \item \texttt{TITLE-ABS-KEY( ("Data Distribution Service" ) OR (iot AND middleware ) OR (mqtt OR ("Message Queuing Telemetry Transport") ) OR ("SOME/IP") ) AND ( vehicular OR ("software defined vehicle") OR automotive OR car )}, which resulted in 172 entries.
    \item \texttt{TITLE-ABS-KEY ( ((container AND (orchestration OR virtualization) ) OR (workload AND (orchestration OR virtualization) ) OR ( software AND (orchestration OR virtualization) ) OR (Kubernetes) ) AND ( vehicular OR ( software AND defined AND vehicle ) OR automotive OR car ) )}, which resulted in 350 entries. %2
    \item \texttt{TITLE-ABS-KEY(( ("Data Distribution Service" ) OR (iot AND middleware ) OR (mqtt OR ("Message Queuing Telemetry Transport" )) OR ("SOME/IP" ) ) AND ( TSN OR ("Time Sensitive Network") OR (DetNet) OR ("Deterministic Networks")) )}, which resulted in 10 entries. %3
\end{itemize}
}
\normalsize
These queries provided the results obtained detailed in~fig.~\ref{fig:sota-methodology}. %summarized in~\cref{tab:sota-methodology}

% \begin{table}[!htp]
%     \centering
%     \caption{Overview of the selection process — $n$ for each initial query}
    
%     \resizebox{\textwidth}{!}{%
%     \begin{tabular}{lp{0.25\linewidth}p{0.25\linewidth}p{0.3\linewidth}p{0.3\linewidth}}
%     \toprule
    
%     \textbf{Query} & \textbf{$n$ initial} & \textbf{$n$ excluded} & \textbf{$n$ selected (manually)} & $n$ \textbf{read} \\
%     \midrule
%     1     & 419       & 69         &   21                     &  18     \\
%     \midrule
%      2     & 207       & 35         &  60                     & 60      \\
%     \midrule
%      3     & 10        & 0          &  10                     & 10      \\
%     \bottomrule
%     \end{tabular}%
%     }
%     \label{tab:sota-methodology}
% \end{table}

\begin{figure}[!ht]
    \centering
    
    \begin{subfigure}[b]{0.8\textwidth}
         \centering
         \includegraphics[width=\columnwidth]{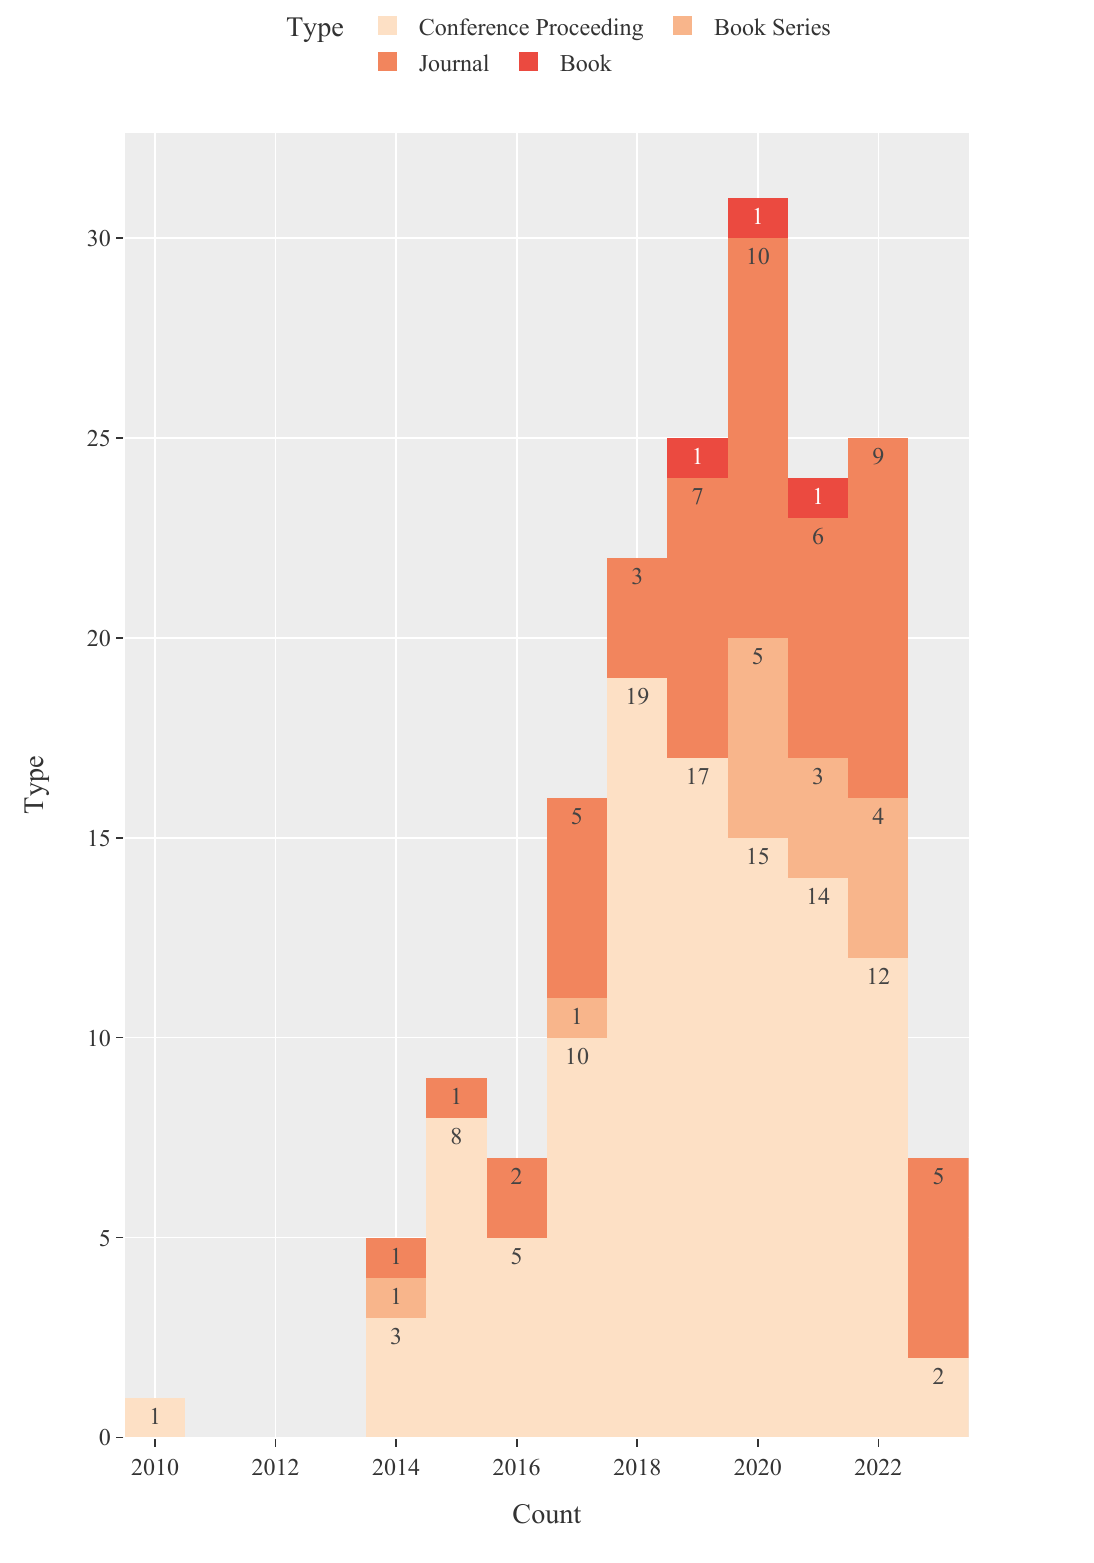}
         
         \caption[Number of obtained titles per year for query 1]{Number of obtained titles per year for query 1.}
     \end{subfigure}
\end{figure}

\begin{figure}[!ht]
    \ContinuedFloat
    \centering
    \begin{subfigure}[b]{0.8\textwidth}
        \centering
        \includegraphics[width=\columnwidth]{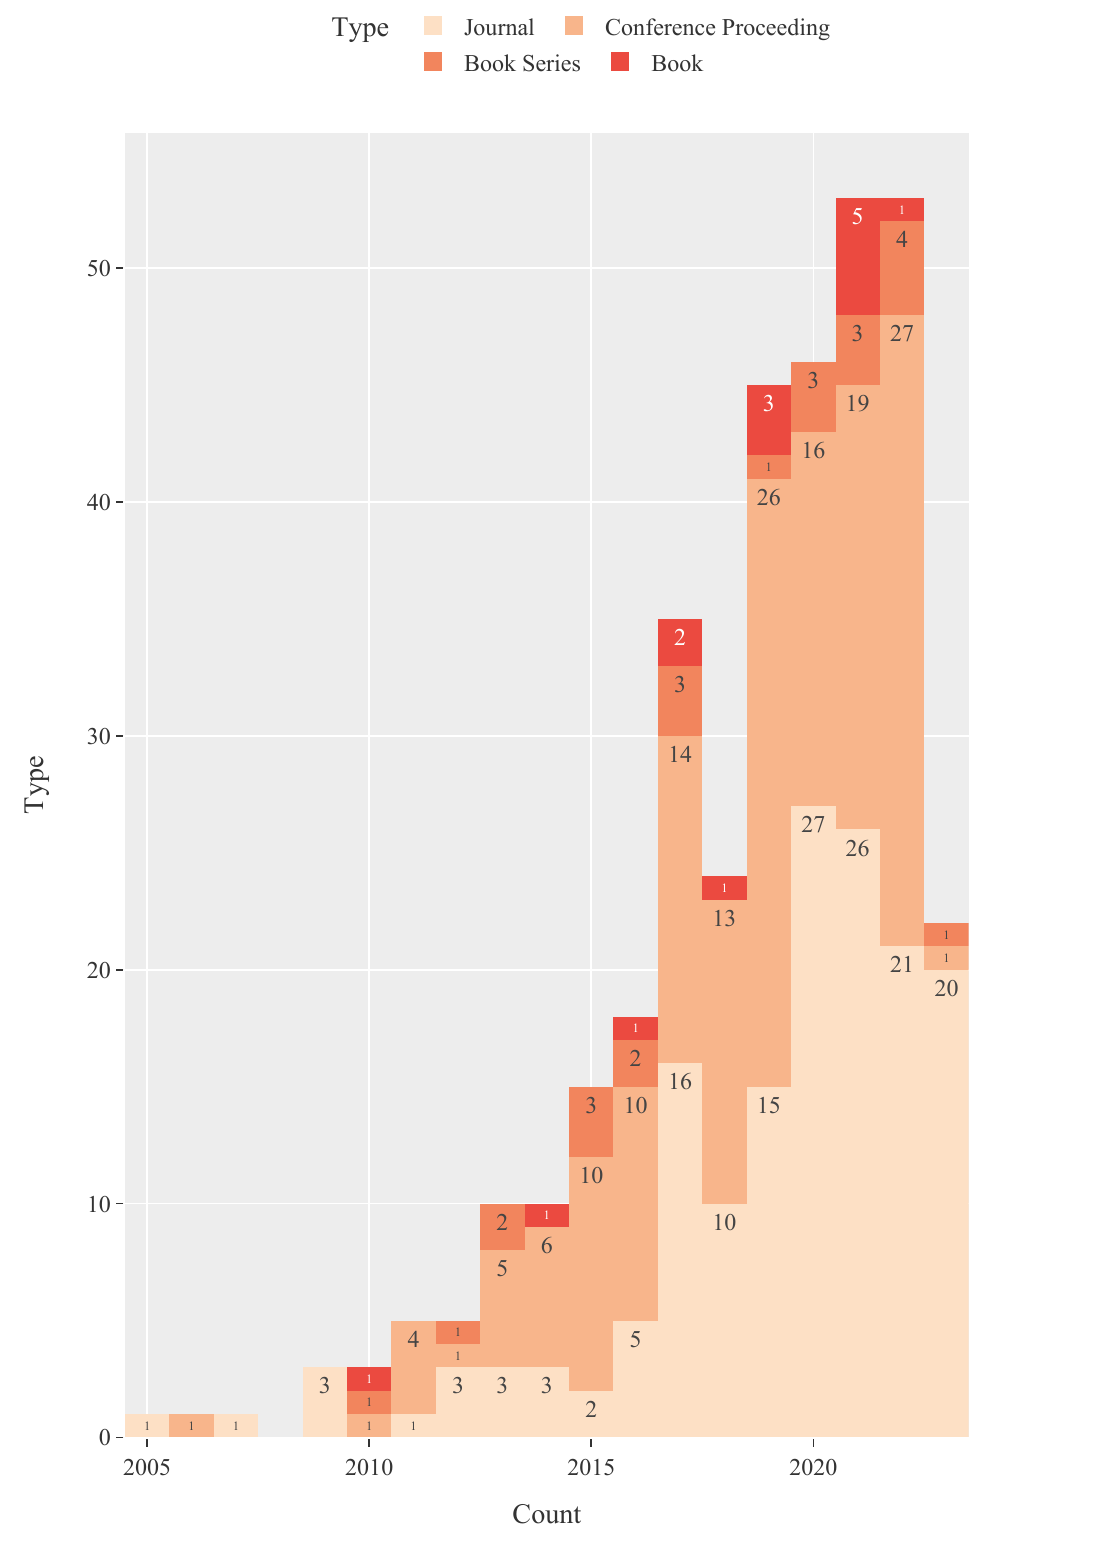}
        \label{fig:sota-methodology-year-2}
        \caption[Number of obtained titles per year for query 2]{Number of obtained titles per year for query 2.}
    \end{subfigure}
\end{figure}

\begin{figure}[!ht]
    \ContinuedFloat
    \centering
    \begin{subfigure}[b]{0.8\textwidth}
        \includegraphics[width=\columnwidth]{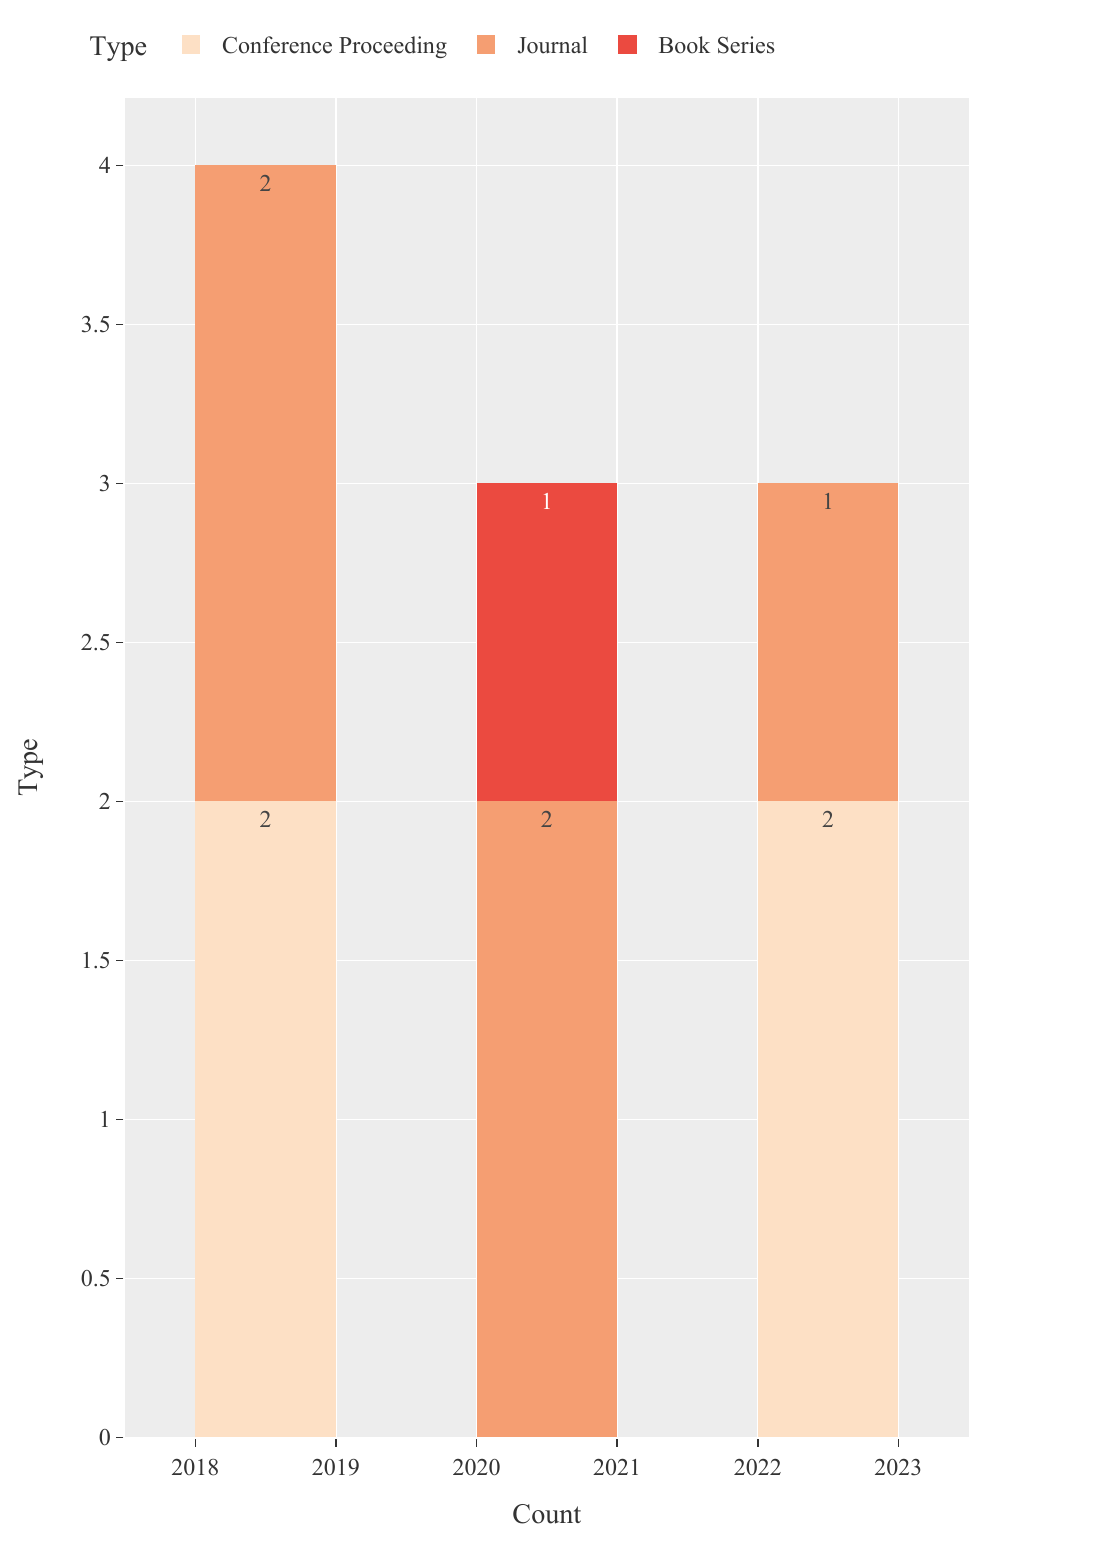}
        \label{fig:sota-methodology-year-3}
        \caption[Number of obtained titles per year for query 3]{Number of obtained titles per year for query 3.} 
    \end{subfigure}
    \caption[Results of executed systematic researches across the years]{Results of executed systematic researches across the years.}
    \label{fig:sota-methodology}
\end{figure}

From this \textbf{preliminary} set of readings, the relevant references were considered for a second phase of readings, with the final statistics in~fig.~\ref{fig:appendix-methodology-year} and~fig.~\ref{fig:appendix-methodology-type}.

\begin{figure}[!ht]
    \centering
    \begin{subfigure}[t]{0.45\columnwidth}
        \includegraphics[width=\columnwidth]{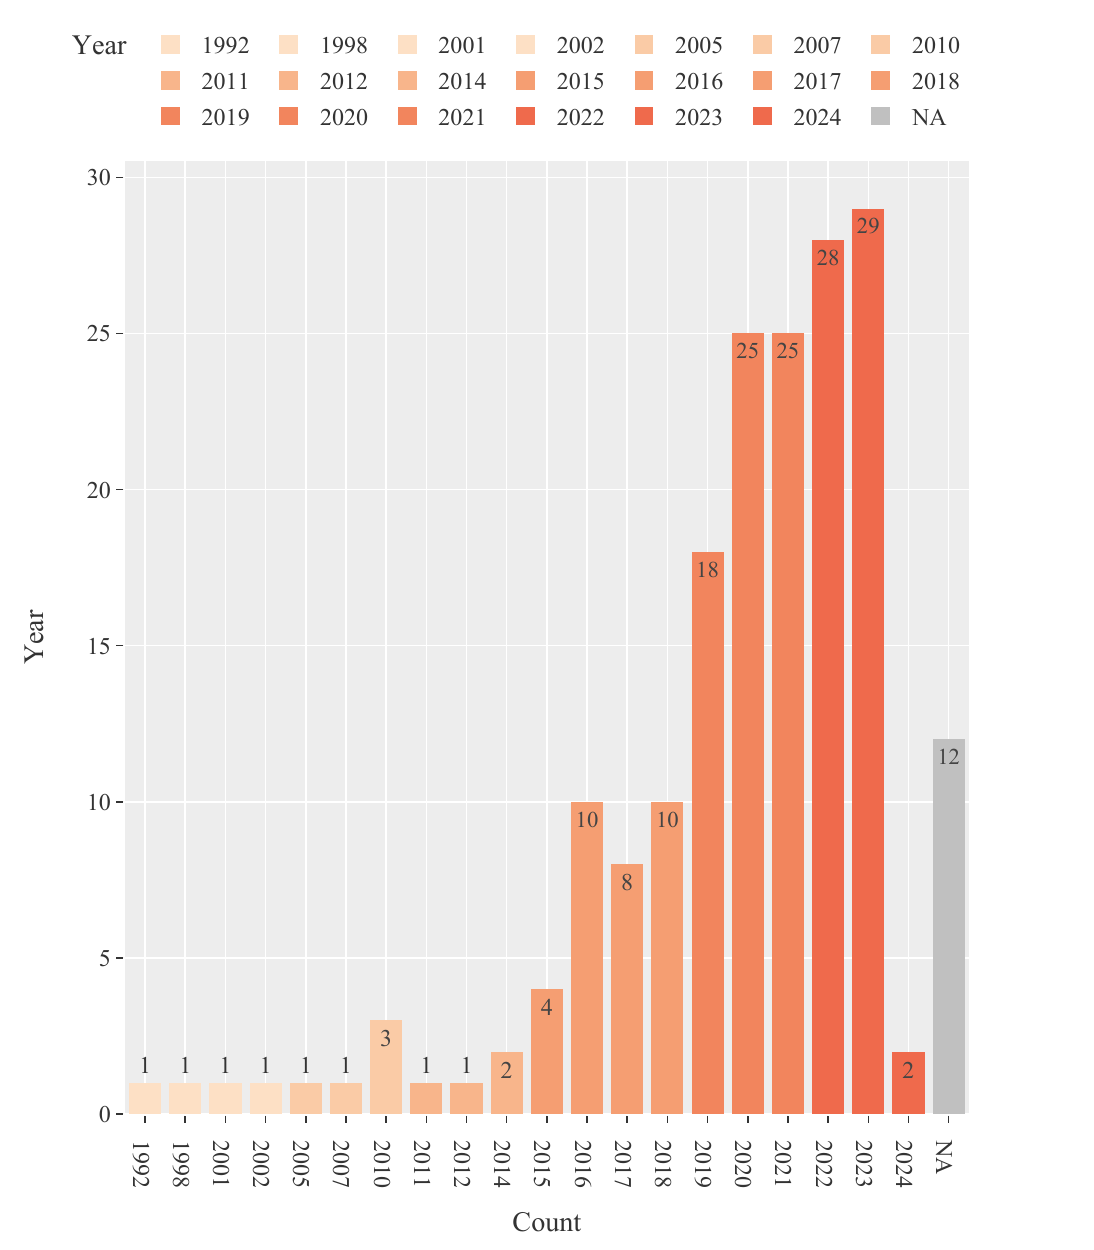}
        \caption{Overview.}  
    \end{subfigure}
    ~
    \begin{subfigure}[t]{0.45\columnwidth}
        \includegraphics[width=\columnwidth]{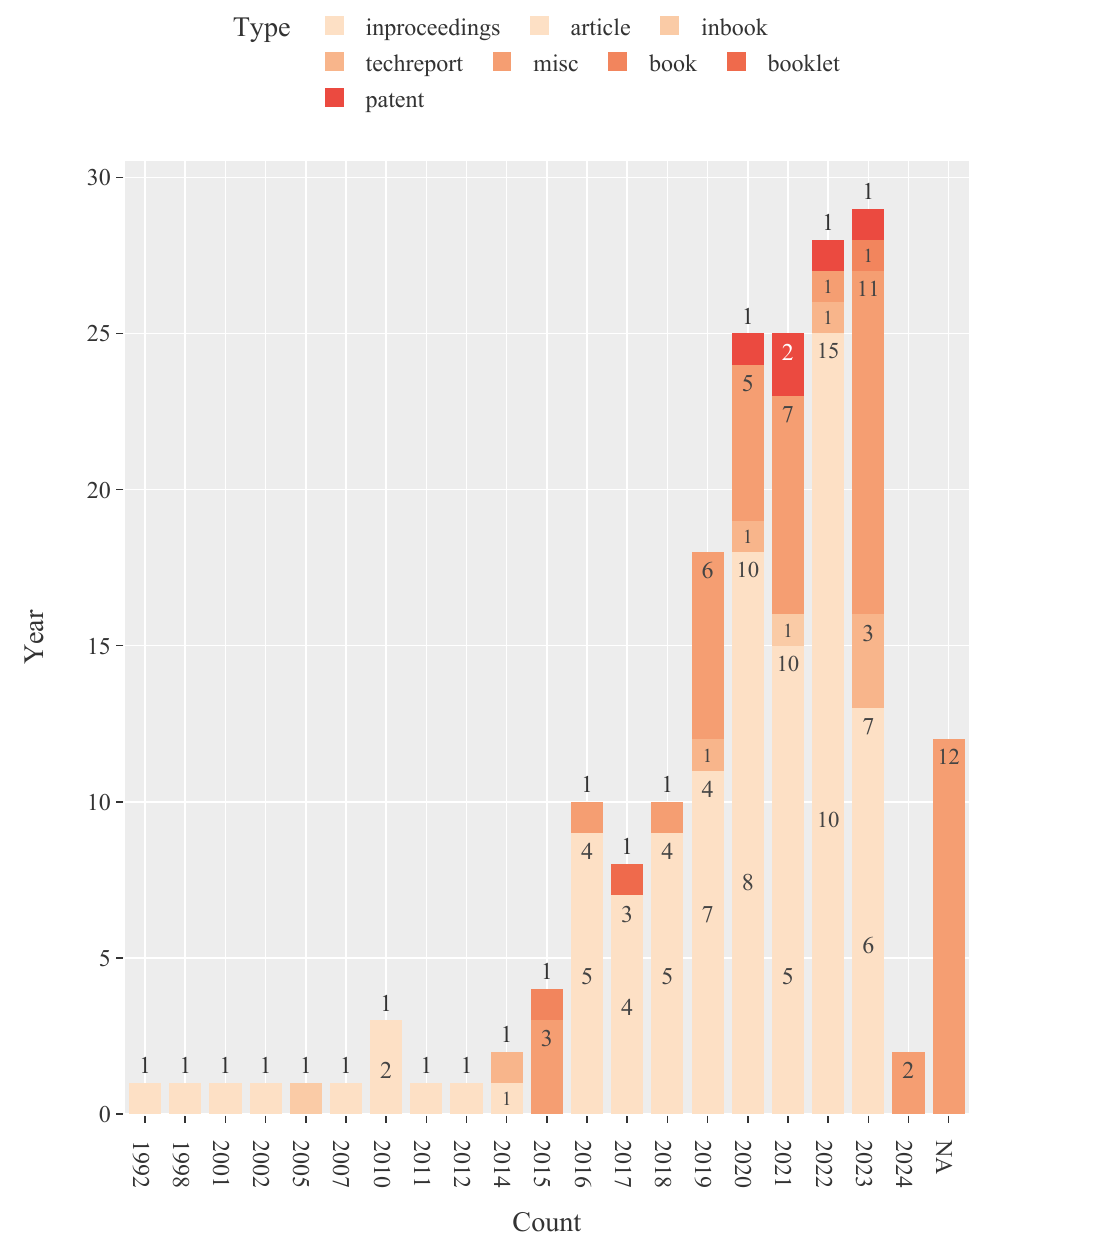}
        \caption{Detailed view per type.}  
    \end{subfigure}    
    \caption[Statistics on the read literature per year]{Statistics on the read literature per year.} 
    \label{fig:appendix-methodology-year} 
\end{figure}

\begin{figure}[!ht]
\centering
    \begin{subfigure}[t]{0.45\columnwidth}
        \includegraphics[width=\columnwidth]{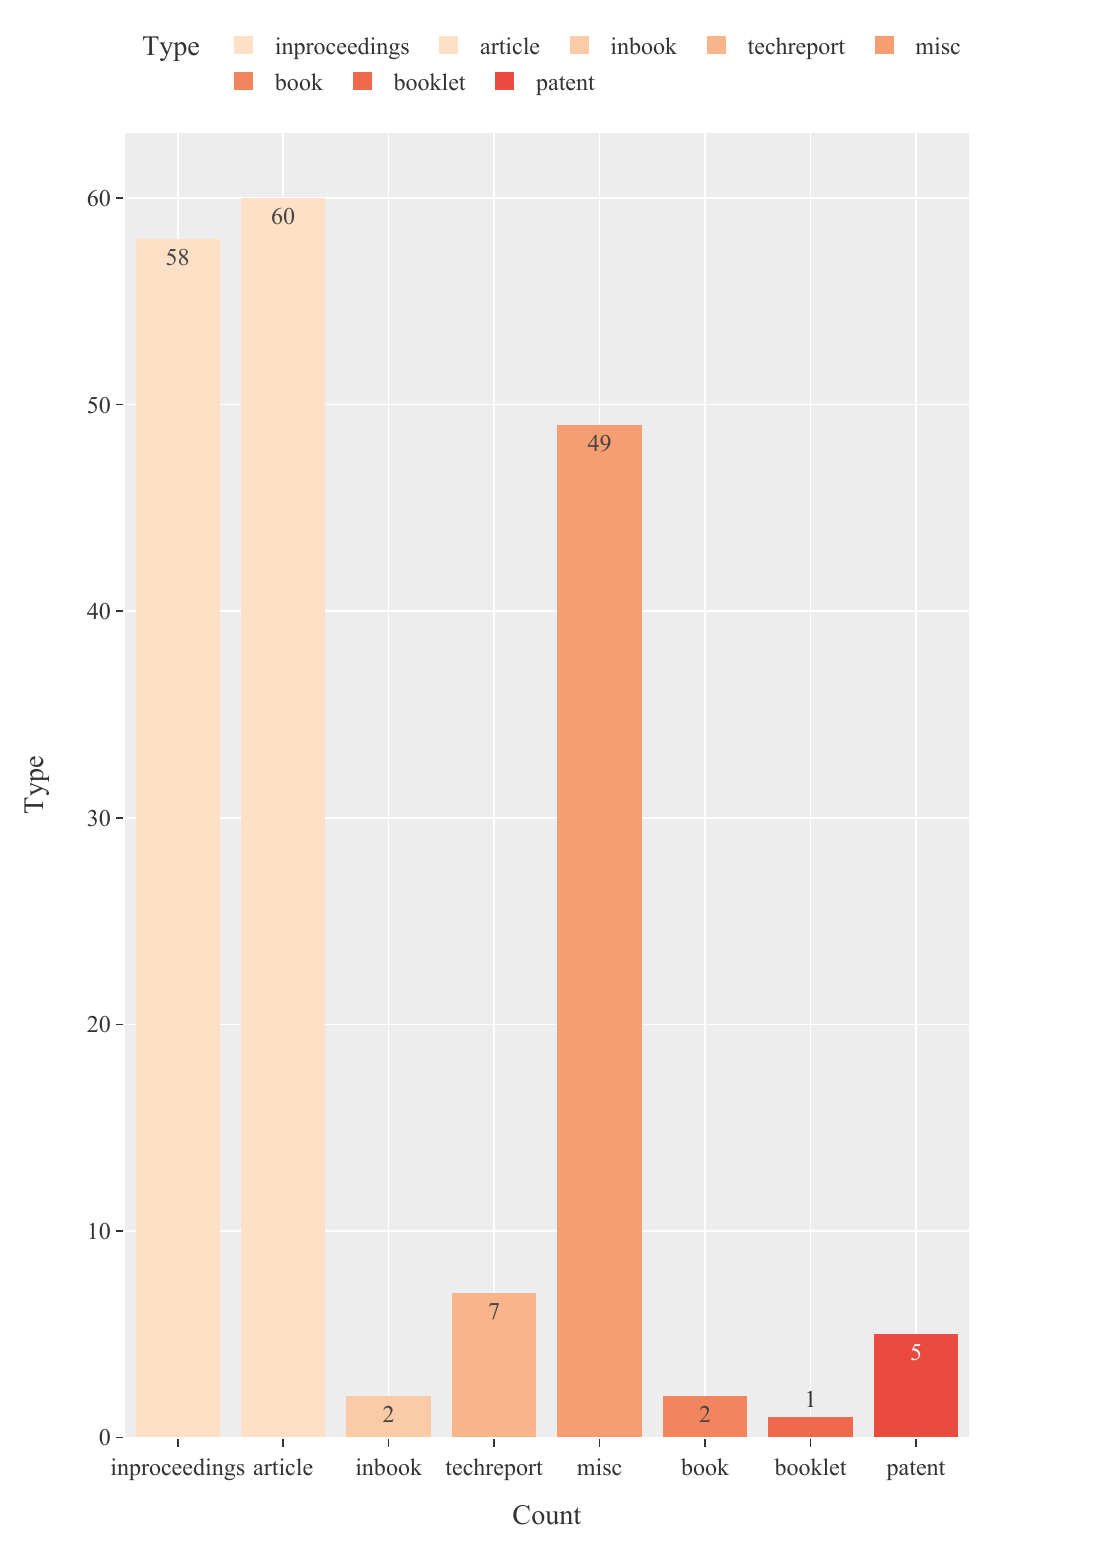}
        \caption{Overview.}  
    \end{subfigure}
    ~
    \begin{subfigure}[t]{0.45\columnwidth}
        \includegraphics[width=\columnwidth]{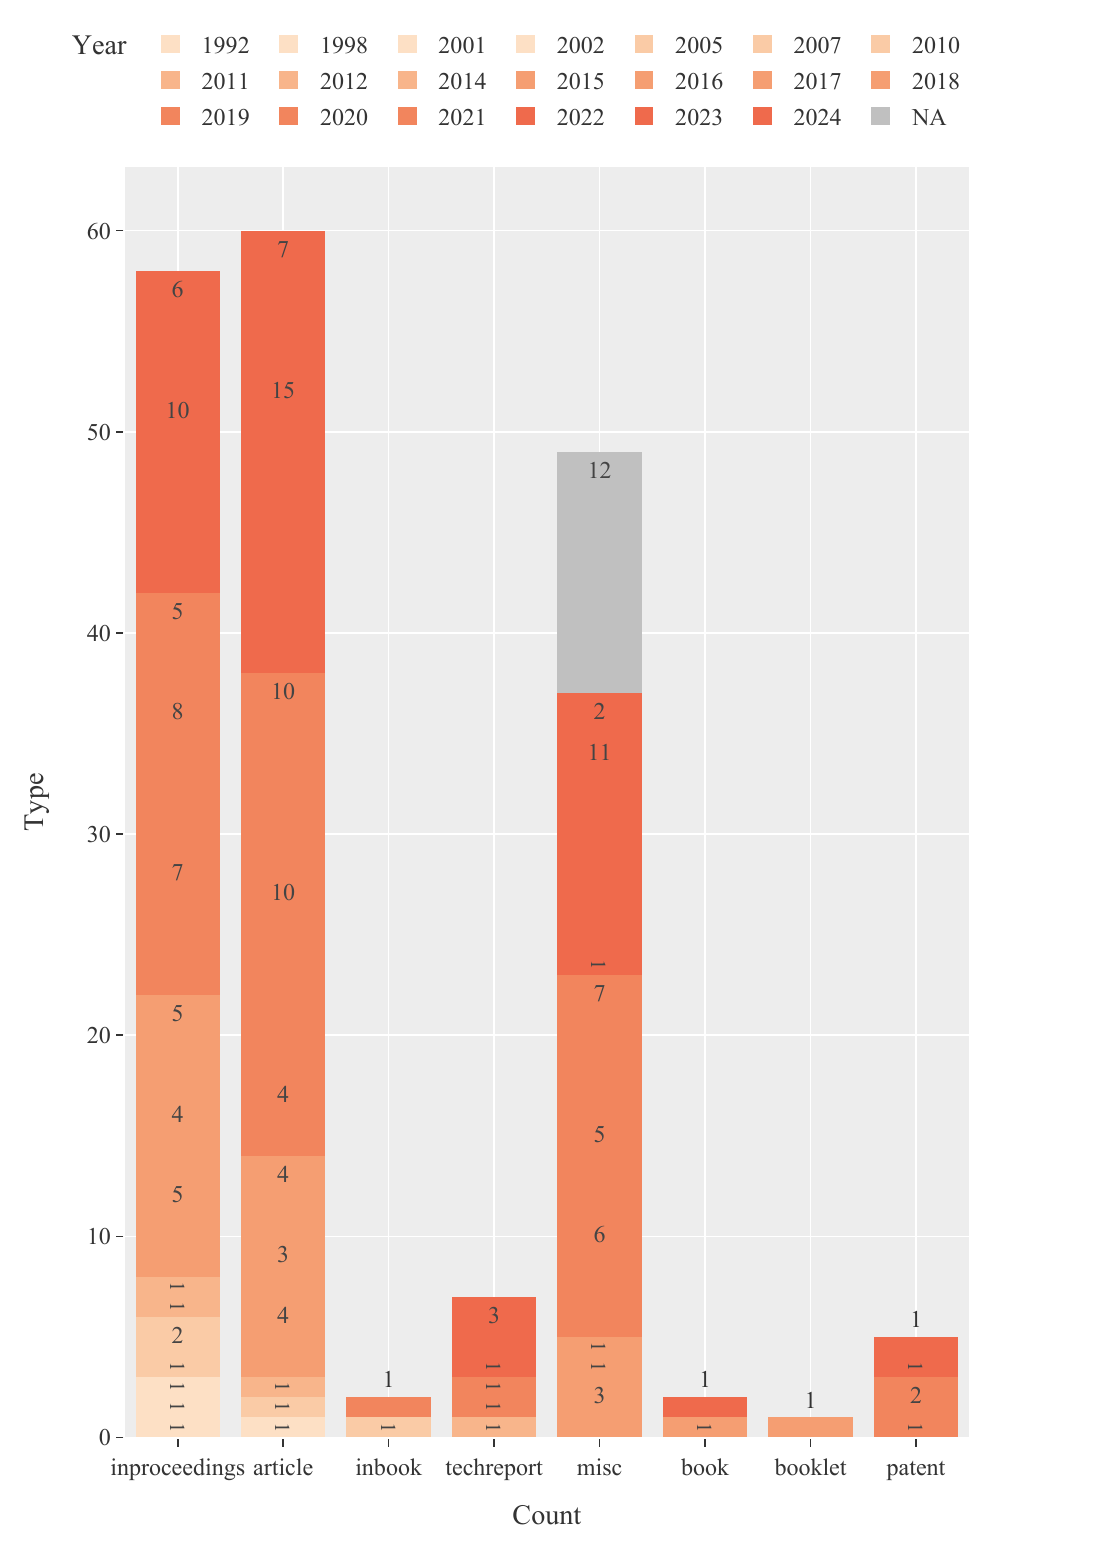}
        \caption{Detailed view per year.}  
    \end{subfigure}    
    \caption[Statistics on the read literature per type]{Statistics on the read literature per type.}
    \label{fig:appendix-methodology-type} 
\end{figure}

These statistics show an emphasis in articles and in proceedings from later years — up to 2023, the year the initial research was conducted — without ignoring a well needed historical perspective. In addition, it shall be emphasized the usage of references within \textit{misc} category — \ie \texit{gray literature} such as white-papers, websites, developer documentation, videos — which was essential to ensure the industrial automaker landscape (which does not tend to publish peer-reviewed articles) was properly covered.

%%%%%%%%%%%%%%%%%%%%%%%%%%
\chapter{DDS-TSN configuration example}
\label{appendix:dds-tsn-example}
\footnotesize {
\begin{code}
\inputminted{json}{chapters/res/dds-tsn-example.json}
\caption[\acs*{dds}-\acs*{tsn} configuration example]{\acs*{dds}-\acs*{tsn} configuration example.}
\end{code}
}
%%%%%%%%%%%%%%%%%%%%%%%%%%
\chapter{Current architecture}
\label{appendix:supreme-arch}
\normalsize
The current version of the architecture considers both the work depicted in~fig.~\ref{fig:arch} and posterior discussions with the author of~\cite{lopes2023time}.

\begin{figure}[!ht]
\centering
%\includesvg[scale=0.5]{figs/arch/Supreme-Controller.svg}
\includegraphics[width=0.9\columnwidth]{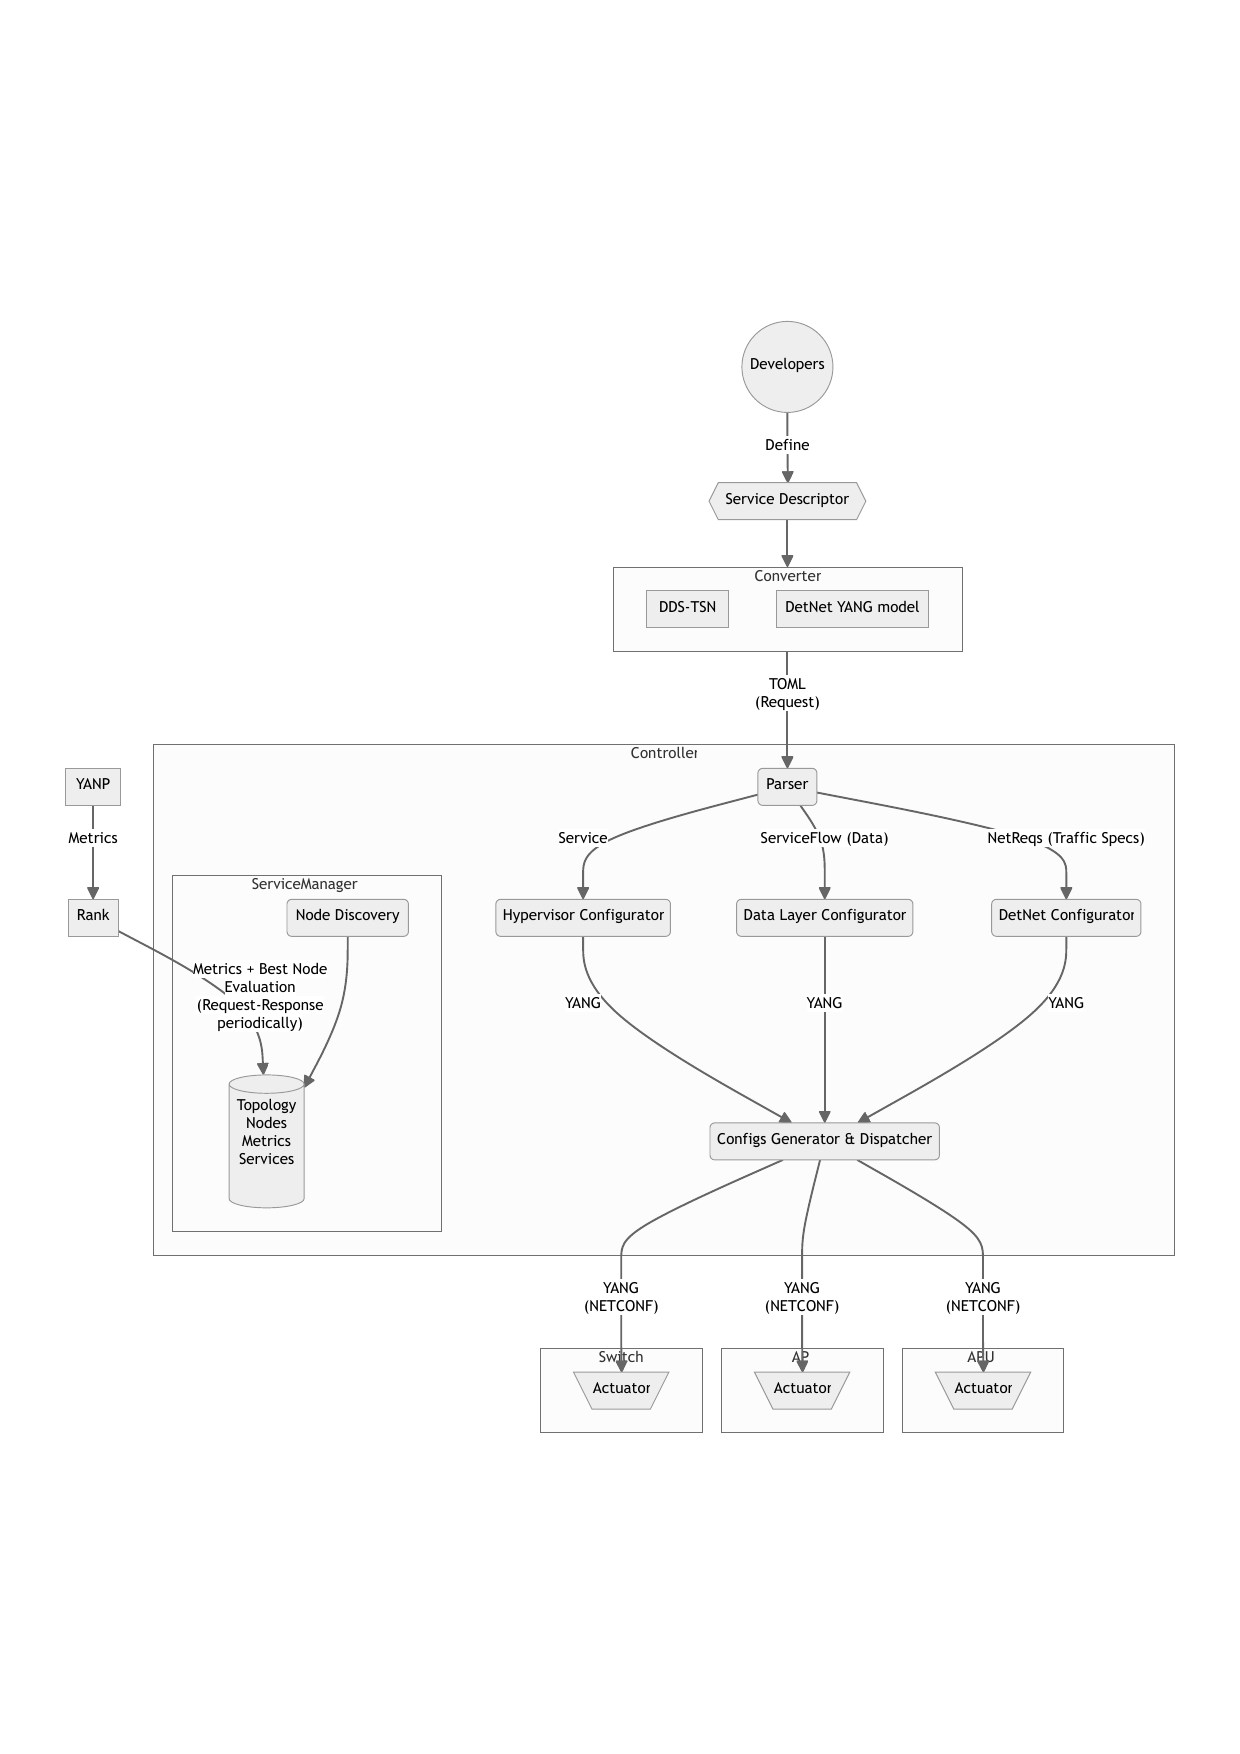}
\caption[Current architecture of the controller]{Current architecture of the controller.}
\end{figure}

The main differences are related to the integration of existing tools such as YANP — Yet Another Network Profiler, with the goal of obtaining some metrics from network connections, such as bandwidth, delay, jitter, packet loss, in both active and passive way — and the Rank protocol — supporting a node  self-assessment by request of a fully-distributed resource allocation protocol — and the choice of standard for configuration of devices — with the usage of \ac{netconf} with \ac{yang} models.

%%%%%%%%%%%%%%%%%%%%%%%%%%
\chapter{Current service descriptor and topology descriptor}
\label{appendix:service-descriptor}

\footnotesize {
\begin{code}

\inputminted{toml}{chapters/res/service-descriptor.toml}
\caption[Example of the current service descriptor]{Example of the current service descriptor.}
\end{code}

\begin{code}
\footnotesize {\inputminted{toml}{chapters/res/topology-descriptor.toml}}
\caption[Example of the current topology descriptor]{Example of the current topology descriptor.}
\end{code}
}

%%%%
% Empty page
\newpage
\thispagestyle{empty}
\mbox{} \vfill \centering \Large{This page was intentionally left blank} \vfill \mbox{}
